# Supplementary material for: A Reexamination of the COnfLUX 2.5D LU Factorization Algorithm
Source: arXiv:2404.06713 source file (2024-04-10)
Supplement: Supplementary file 1 [file appendix.tex]

\secput{app}{Artifact Description}
\punt{% begin punt
Following is some paragraph for a research paper. Please polish it appropriate. Making it concise, clear, and to-the-point. You should NOT omit any main information. You should also keep all the Latex commands of the input.
}% end punt

In the main text of this 4-page comment paper, we provide citations for all evidence and sources. The original paper by Kwasniewski et al. \cite{KwasniewskiKaBe21} can be accessed at the ACM Digital Library. Additionally, the code base we analyzed is available at the GitHub repository: \href{https://github.com/eth-cscs/conflux}{https://github.com/eth-cscs/conflux}. It is important to note that our examination focused on the snapshot from May 29, 2023, while the original paper was published in SC'21.
